# Supplementary material for: Tensor Decompositions for Count Data that Leverage Stochastic and Deterministic Optimization
Source: arXiv:2207.14341 source file (2024-07-12)
Supplement: Supplementary file 1 [file content_background_supplementary.tex]

In prior
work~\cite{Myers20ParameterSensitivityAnalysis,Myers21UsingComputationEffectively},
we showed that both GCP and CPAPR are sensitive to hyperparameters. The
parameter space for GCP-Adam is especially large and tuning is difficult. In
preliminary experiments on real data, we noted dismal performance of GCP
compared to CPAPR,\footnote{From 20 random starts, CPAPR computed solutions
equal to the empirical MLE seven times (35\%); the median time to solution was
842 seconds. On the other hand, GCP worked $2.2\times$ longer in the median case
(1,837 seconds), converging in zero instances.} which we attribute to the use of
default software parameters. In private correspondence,\footnote{T.G. Kolda,
email to author, March 8, 2021.} the authors of GCP discouraged using default
parameters. In these experiments and other preliminary work, we observed the
number of nonzero and zero entries sampled for function evaluations and gradient
computations to be especially impactful. For the experimental results presented
in this work, we typically sample at least 90\% of nonzero and zero entries. The
reason for this is two-fold. Firstly, we want to understand the expected
behavior of GCP as a standalone solver and as a subroutine of \textsc{HybridGC}.
By sampling a large number of nonzero and zero entries, we establish a heuristic
upper bound on algorithm effectiveness. Lastly, we are only concerned with the
proof of concept of \textsc{HybridGC} at present. We leave performance studies
and optimizations to future work.

One common approach to parameter tuning is exhaustive search through a
discretized grid of parameter values. This approach is reasonable for CPAPR
since it has relatively few tunable parameters. However, exhaustive search is
infeasible for GCP. One practical option for hyperparameter tuning is Latin
hypercube sampling~\cite{Helton03LatinHypercubeSampling}, which has not gained
much attention in the machine learning community. Since a proper investigation
is beyond the scope of this work, we leave this direction to future research.
